# Supplementary material for: Comparative Bi-stochastizations and Associated Clusterings/Regionalizations of the 1995-2000 U. S. Intercounty Migration Network
Source: arXiv:1208.3428 source file (2012-09-14)
Supplement: Supplementary file 1 [file SupplementalMaterial.pdf]

**Supplemental Material**

**A. Mathematica Code provided by Michael Trott implementing WLK-algorithm used to obtain the squared-norm-bi-stochastic matrix.**
**The input dataset "INTERCOUNTYFLOWS" is a 735,531-long list of the non-zero flows, that is, {county number, county number j, migration flow}. 175,000 iterations of the algorithm were run to produce the squared-norm-bi-stochastic table ("G") analyzed. The sum-of-squares difference between the (3,107)^2 entries at the 174,999 and 175,000 steps was 4.85 x 10^{-36}, indicative of strong convergence.**

```
n = 3107;
G = Developer`ToPackedArray@
  Normal@SparseArray[({#1, #2} -> 1. #3) & @@@ Get["INTERCOUNTYFLOWS"]];

P = Developer`ToPackedArray@Array[1. &, n];
id = Developer`ToPackedArray@(1. IdentityMatrix[n]);

Do[y1 = Array[Evaluate[P.G/n] &, n] - G;
 b6 = (id + y1).P;
 b7 = Transpose[Array[Evaluate[b6/n] &, n]];
 AT = b7 - y1;
 G = (AT + Abs[AT])/2., {j, 1, 175000}]
```

**B. Intrastate Pairs (Strong Component Doublets)**

{{1,{Baldwin, AL,Mobile, AL}},{2,{Blount, AL,Cullman, AL}}}
{{3,{Calhoun, AL,Talladega, AL}},{4,{Coffee, AL,Dale, AL}}}
{{5,{Colbert, AL,Lauderdale, AL}},{6,{Coosa, AL,Tallapoosa, AL}}}
{{7,{DeKalb, AL,Jackson, AL}},{8,{Elmore, AL,Montgomery, AL}}}
{{9,{Etowah, AL,Marshall, AL}},{10,{Jefferson, AL,Shelby, AL}}}
{{11,{Lawrence, AL,Morgan, AL}},{12,{Lee, AL,Russell, AL}}}
{{13,{Limestone, AL,Madison, AL}},{14,{Anchorage, AK,Matanuska-Susitna, AK}}}
{{15,{Bethel, AK,Wade Hampton, AK}},{16,{Fairbanks North Star, AK,Yukon-Koyukuk, AK}}}
{{17,{Ketchikan Gateway, AK,Prince of Wales-Outer Ketchikan, AK}},{18,{Southeast Fairbanks, AK,Valdez-Cordova, AK}}}
{{19,{Apache, AZ,Navajo, AZ}},{20,{Graham, AZ,Greenlee, AZ}}}
{{21,{Arkansas, AR,Prairie, AR}},{22,{Baxter, AR,Marion, AR}}}
{{23,{Benton, AR,Washington, AR}},{24,{Boone, AR,Newton, AR}}}
{{25,{Calhoun, AR,Dallas, AR}},{26,{Clay, AR,Greene, AR}}}
{{27,{Conway, AR,Perry, AR}},{28,{Craighead, AR,Poinsett, AR}}}
{{29,{Crawford, AR,Sebastian, AR}},{30,{Garland, AR,Hot Spring, AR}}}
{{31,{Hempstead, AR,Nevada, AR}},{32,{Independence, AR,Sharp, AR}}}
{{33,{Jackson, AR,Woodruff, AR}},{34,{Lawrence, AR,Randolph, AR}}}
{{35,{Pope, AR,Yell, AR}},{36,{Pulaski, AR,Saline, AR}}}
{{37,{Searcy, AR,Van Buren, AR}},{38,{Amador, CA,Calaveras, CA}}}
{{39,{Butte, CA,Glenn, CA}},{40,{Fresno, CA,Madera, CA}}}
{{41,{Inyo, CA,Mono, CA}},{42,{Lassen, CA,Plumas, CA}}}
{{43,{Los Angeles, CA,Orange, CA}},{44,{Marin, CA,Sonoma, CA}}}
{{45,{Monterey, CA,Santa Cruz, CA}},{46,{Placer, CA,Sacramento, CA}}}
{{47,{Shasta, CA,Tehama, CA}},{48,{Sutter, CA,Yuba, CA}}}
{{49,{Adams, CO,Jefferson, CO}},{50,{Alamosa, CO,Conejos, CO}}}
{{51,{Arapahoe, CO,Denver, CO}},{52,{Delta, CO,Montrose, CO}}}
{{53,{Larimer, CO,Weld, CO}},{54,{Moffat, CO,Routt, CO}}}
{{55,{Ouray, CO,San Miguel, CO}},{56,{Rio Grande, CO,Saguache, CO}}}
{{57,{Washington, CO,Yuma, CO}},{58,{Hartford, CT,Tolland, CT}}}
{{59,{New London, CT,Windham, CT}},{60,{Kent, DE,Sussex, DE}}}
{{61,{Brevard, FL,Indian River, FL}},{62,{Calhoun, FL,Liberty, FL}}}
{{63,{Charlotte, FL,DeSoto, FL}},{64,{Clay, FL,Duval, FL}}}
{{65,{Collier, FL,Lee, FL}},{66,{Columbia, FL,Suwannee, FL}}}
{{67,{Escambia, FL,Santa Rosa, FL}},{68,{Gilchrist, FL,Levy, FL}}}
{{69,{Glades, FL,Hendry, FL}},{70,{Hardee, FL,Highlands, FL}}}
{{71,{Hillsborough, FL,Pinellas, FL}},{72,{Manatee, FL,Sarasota, FL}}}
{{73,{Okaloosa, FL,Walton, FL}},{74,{Orange, FL,Seminole, FL}}}

{{75,{Atkinson, GA,Coffee, GA}},{76,{Bartow, GA,Gordon, GA}}}
{{77,{Ben Hill, GA,Irwin, GA}},{78,{Bibb, GA,Jones, GA}}}
{{79,{Brooks, GA,Lowndes, GA}},{80,{Burke, GA,Jenkins, GA}}}
{{81,{Chatham, GA,Effingham, GA}},{82,{Clarke, GA,Oconee, GA}}}
{{83,{Clinch, GA,Lanier, GA}},{84,{Columbia, GA,Richmond, GA}}}
{{85,{Coweta, GA,Fayette, GA}},{86,{Crisp, GA,Dooly, GA}}}
{{87,{Decatur, GA,Seminole, GA}},{88,{Dougherty, GA,Lee, GA}}}
{{89,{Grady, GA,Thomas, GA}},{90,{Harris, GA,Muscogee, GA}}}
{{91,{Houston, GA,Peach, GA}},{92,{Lincoln, GA,Wilkes, GA}}}
{{93,{McDuffie, GA,Warren, GA}},{94,{Madison, GA,Oglethorpe, GA}}}
{{95,{Montgomery, GA,Toombs, GA}},{96,{Murray, GA,Whitfield, GA}}}
{{97,{Newton, GA,Rockdale, GA}},{98,{Schley, GA,Sumter, GA}}}
{{99,{Stewart, GA,Webster, GA}},{100,{Hawaii, HI,Honolulu, HI}}}
{{101,{Kauai, HI,Maui, HI}},{102,{Ada, ID,Canyon, ID}}}
{{103,{Bannock, ID,Bingham, ID}},{104,{Boise, ID,Gem, ID}}}
{{105,{Bonner, ID,Kootenai, ID}},{106,{Bonneville, ID,Jefferson, ID}}}
{{107,{Cassia, ID,Minidoka, ID}},{108,{Elmore, ID,Owyhee, ID}}}
{{109,{Fremont, ID,Madison, ID}},{110,{Gooding, ID,Lincoln, ID}}}
{{111,{Idaho, ID,Lewis, ID}},{112,{Jerome, ID,Twin Falls, ID}}}
{{113,{Boone, IL,Winnebago, IL}},{114,{Carroll, IL,Stephenson, IL}}}
{{115,{Christian, IL,Shelby, IL}},{116,{Clark, IL,Edgar, IL}}}
{{117,{Clay, IL,Wayne, IL}},{118,{Clinton, IL,Marion, IL}}}
{{119,{Coles, IL,Cumberland, IL}},{120,{Cook, IL,DuPage, IL}}}
{{121,{Effingham, IL,Fayette, IL}},{122,{Franklin, IL,Williamson, IL}}}
{{123,{Gallatin, IL,Saline, IL}},{124,{Greene, IL,Jersey, IL}}}
{{125,{Iroquois, IL,Kankakee, IL}},{126,{Jackson, IL,Perry, IL}}}
{{127,{Jefferson, IL,Washington, IL}},{128,{Jo Daviess, IL,Dubuque, IA}}}
{{129,{Knox, IL,Warren, IL}},{130,{Lee, IL,Ogle, IL}}}
{{131,{Macoupin, IL,Montgomery, IL}},{132,{Madison, IL,St. Clair, IL}}}
{{133,{Menard, IL,Sangamon, IL}},{134,{Peoria, IL,Tazewell, IL}}}
{{135,{Blackford, IN,Jay, IN}},{136,{Boone, IN,Montgomery, IN}}}
{{137,{Carroll, IN,White, IN}},{138,{Clark, IN,Floyd, IN}}}
{{139,{Clay, IN,Vigo, IN}},{140,{Clinton, IN,Tippecanoe, IN}}}
{{141,{Dearborn, IN,Ripley, IN}},{142,{DeKalb, IN,Steuben, IN}}}
{{143,{Delaware, IN,Madison, IN}},{144,{Elkhart, IN,St. Joseph, IN}}}
{{145,{Fayette, IN,Franklin, IN}},{146,{Fountain, IN,Warren, IN}}}
{{147,{Fulton, IN,Pulaski, IN}},{148,{Gibson, IN,Pike, IN}}}
{{149,{Grant, IN,Wabash, IN}},{150,{Greene, IN,Sullivan, IN}}}
{{151,{Hancock, IN,Henry, IN}},{152,{Huntington, IN,Wells, IN}}}
{{153,{Jasper, IN,Newton, IN}},{154,{Jefferson, IN,Scott, IN}}}
{{155,{Lake, IN,Porter, IN}},{156,{Ohio, IN,Switzerland, IN}}}
{{157,{Parke, IN,Vermillion, IN}},{158,{Perry, IN,Spencer, IN}}}
{{159,{Vanderburgh, IN,Warrick, IN}},{160,{Adair, IA,Guthrie, IA}}}
{{161,{Adams, IA,Taylor, IA}},{162,{Allamakee, IA,Winneshiek, IA}}}
{{163,{Audubon, IA,Cass, IA}},{164,{Buchanan, IA,Fayette, IA}}}
{{165,{Buena Vista, IA,Sac, IA}},{166,{Cerro Gordo, IA,Worth, IA}}}
{{167,{Chickasaw, IA,Floyd, IA}},{168,{Clarke, IA,Decatur, IA}}}
{{169,{Clay, IA,Dickinson, IA}},{170,{Clinton, IA,Jackson, IA}}}
{{171,{Davis, IA,Wapello, IA}},{172,{Franklin, IA,Hardin, IA}}}
{{173,{Fremont, IA,Page, IA}},{174,{Hancock, IA,Winnebago, IA}}}
{{175,{Howard, IA,Mitchell, IA}},{176,{Jasper, IA,Poweshiek, IA}}}
{{177,{Jefferson, IA,Van Buren, IA}},{178,{Louisa, IA,Muscatine, IA}}}
{{179,{Lyon, IA,Sioux, IA}},{180,{Mahaska, IA,Marion, IA}}}
{{181,{Marshall, IA,Tama, IA}},{182,{Mills, IA,Pottawattamie, IA}}}
{{183,{O'Brien, IA,Osceola, IA}},{184,{Anderson, KS,Franklin, KS}}}
{{185,{Butler, KS,Sedgwick, KS}},{186,{Chautauqua, KS,Elk, KS}}}
{{187,{Cherokee, KS,Crawford, KS}},{188,{Cloud, KS,Republic, KS}}}
{{189,{Coffey, KS,Lyon, KS}},{190,{Cowley, KS,Sumner, KS}}}
{{191,{Harvey, KS,Marion, KS}},{192,{Leavenworth, KS,Wyandotte, KS}}}
{{193,{Linn, KS,Miami, KS}},{194,{Logan, KS,Thomas, KS}}}
{{195,{McPherson, KS,Reno, KS}},{196,{Osage, KS,Shawnee, KS}}}
{{197,{Ottawa, KS,Saline, KS}},{198,{Pottawatomie, KS,Riley, KS}}}
{{199,{Adair, KY,Russell, KY}},{200,{Boone, KY,Kenton, KY}}}
{{201,{Bourbon, KY,Nicholas, KY}},{202,{Boyd, KY,Greenup, KY}}}
{{203,{Bullitt, KY,Jefferson, KY}},{204,{Caldwell, KY,Lyon, KY}}}

{{205,{Calloway, KY,Graves, KY}},{206,{Carroll, KY,Trimble, KY}}}
{{207,{Clark, KY,Powell, KY}},{208,{Clay, KY,Leslie, KY}}}
{{209,{Crittenden, KY,Livingston, KY}},{210,{Daviess, KY,Ohio, KY}}}
{{211,{Fayette, KY,Jessamine, KY}},{212,{Fleming, KY,Lewis, KY}}}
{{213,{Green, KY,Taylor, KY}},{214,{Harlan, KY,Letcher, KY}}}
{{215,{Henderson, KY,Union, KY}},{216,{Hopkins, KY,Webster, KY}}}
{{217,{Knott, KY,Perry, KY}},{218,{Lawrence, KY,Martin, KY}}}
{{219,{Lee, KY,Owsley, KY}},{220,{McCracken, KY,Marshall, KY}}}
{{221,{McLean, KY,Muhlenberg, KY}},{222,{Pulaski, KY,Wayne, KY}}}
{{223,{Assumption, LA,St. Mary, LA}},{224,{Bossier, LA,Caddo, LA}}}
{{225,{Claiborne, LA,Webster, LA}},{226,{Franklin, LA,Richland, LA}}}
{{227,{Grant, LA,Rapides, LA}},{228,{Jefferson, LA,Orleans, LA}}}
{{229,{Lafayette, LA,St. Martin, LA}},{230,{Lafourche, LA,Terrebonne, LA}}}
{{231,{St. Charles, LA,St. John the Baptist, LA}},{232,{Androscoggin, ME,Oxford, ME}}}
{{233,{Cumberland, ME,York, ME}},{234,{Franklin, ME,Piscataquis, ME}}}
{{235,{Kennebec, ME,Somerset, ME}},{236,{Knox, ME,Waldo, ME}}}
{{237,{Lincoln, ME,Sagadahoc, ME}},{238,{Baltimore, MD,Baltimore City, MD}}}
{{239,{Kent, MD,Queen Anne's, MD}},{240,{Wicomico, MD,Worcester, MD}}}
{{241,{Hampden, MA,Hampshire, MA}},{242,{Alcona, MI,Iosco, MI}}}
{{243,{Alpena, MI,Presque Isle, MI}},{244,{Arenac, MI,Ogemaw, MI}}}
{{245,{Bay, MI,Saginaw, MI}},{246,{Berrien, MI,Cass, MI}}}
{{247,{Chippewa, MI,Mackinac, MI}},{248,{Eaton, MI,Ingham, MI}}}
{{249,{Genesee, MI,Lapeer, MI}},{250,{Grand Traverse, MI,Leelanau, MI}}}
{{251,{Gratiot, MI,Isabella, MI}},{252,{Huron, MI,Tuscola, MI}}}
{{253,{Ionia, MI,Montcalm, MI}},{254,{Kalamazoo, MI,Van Buren, MI}}}
{{255,{Kent, MI,Ottawa, MI}},{256,{Mecosta, MI,Osceola, MI}}}
{{257,{Missaukee, MI,Wexford, MI}},{258,{Montmorency, MI,Otsego, MI}}}
{{259,{Muskegon, MI,Oceana, MI}},{260,{Aitkin, MN,Itasca, MN}}}
{{261,{Becker, MN,Otter Tail, MN}},{262,{Benton, MN,Stearns, MN}}}
{{263,{Big Stone, MN,Traverse, MN}},{264,{Blue Earth, MN,Nicollet, MN}}}
{{265,{Brown, MN,Watonwan, MN}},{266,{Cass, MN,Crow Wing, MN}}}
{{267,{Cook, MN,Lake, MN}},{268,{Cottonwood, MN,Jackson, MN}}}
{{269,{Douglas, MN,Pope, MN}},{270,{Freeborn, MN,Mower, MN}}}
{{271,{Goodhue, MN,Wabasha, MN}},{272,{Grant, MN,Stevens, MN}}}
{{273,{Kandiyohi, MN,Swift, MN}},{274,{Lake of the Woods, MN,Roseau, MN}}}
{{275,{McLeod, MN,Meeker, MN}},{276,{Mahnomen, MN,Norman, MN}}}
{{277,{Marshall, MN,Pennington, MN}},{278,{Sherburne, MN,Wright, MN}}}
{{279,{Steele, MN,Waseca, MN}},{280,{Alcorn, MS,Prentiss, MS}}}
{{281,{Amite, MS,Pike, MS}},{282,{Benton, MS,Marshall, MS}}}
{{283,{Carroll, MS,Leflore, MS}},{284,{Choctaw, MS,Webster, MS}}}
{{285,{Claiborne, MS,Warren, MS}},{286,{Clarke, MS,Lauderdale, MS}}}
{{287,{Forrest, MS,Lamar, MS}},{288,{Grenada, MS,Montgomery, MS}}}
{{289,{Harrison, MS,Jackson, MS}},{290,{Itawamba, MS,Lee, MS}}}
{{291,{Jasper, MS,Jones, MS}},{292,{Marion, MS,Walthall, MS}}}
{{293,{Simpson, MS,Smith, MS}},{294,{Andrew, MO,Buchanan, MO}}}
{{295,{Barry, MO,Lawrence, MO}},{296,{Barton, MO,Dade, MO}}}
{{297,{Benton, MO,Pettis, MO}},{298,{Caldwell, MO,Ray, MO}}}
{{299,{Callaway, MO,Cole, MO}},{300,{Camden, MO,Miller, MO}}}
{{301,{Cape Girardeau, MO,Scott, MO}},{302,{Cedar, MO,Vernon, MO}}}
{{303,{Chariton, MO,Linn, MO}},{304,{Christian, MO,Greene, MO}}}
{{305,{Clay, MO,Platte, MO}},{306,{Clinton, MO,DeKalb, MO}}}
{{307,{Cooper, MO,Howard, MO}},{308,{Hickory, MO,Polk, MO}}}
{{309,{Jasper, MO,Newton, MO}},{310,{Maries, MO,Osage, MO}}}
{{311,{Marion, MO,Ralls, MO}},{312,{Moniteau, MO,Morgan, MO}}}
{{313,{Putnam, MO,Sullivan, MO}},{314,{Stone, MO,Taney, MO}}}
{{315,{Texas, MO,Wright, MO}},{316,{Beaverhead, MT,Madison, MT}}}
{{317,{Blaine, MT,Hill, MT}},{318,{Fergus, MT,Judith Basin, MT}}}
{{319,{Gallatin, MT,Park, MT}},{320,{Jefferson, MT,Lewis and Clark, MT}}}
{{321,{Missoula, MT,Ravalli, MT}},{322,{Pondera, MT,Teton, MT}}}
{{323,{Adams, NE,Clay, NE}},{324,{Boone, NE,Nance, NE}}}
{{325,{Burt, NE,Washington, NE}},{326,{Cass, NE,Otoe, NE}}}
{{327,{Cedar, NE,Knox, NE}},{328,{Cuming, NE,Thurston, NE}}}
{{329,{Dixon, NE,Wayne, NE}},{330,{Dodge, NE,Saunders, NE}}}
{{331,{Douglas, NE,Sarpy, NE}},{332,{Fillmore, NE,York, NE}}}

{{333,{Franklin, NE,Webster, NE}},{334,{Gage, NE,Jefferson, NE}}}
{{335,{Hall, NE,Howard, NE}},{336,{Hamilton, NE,Merrick, NE}}}
{{337,{Hitchcock, NE,Red Willow, NE}},{338,{Lancaster, NE,Seward, NE}}}
{{339,{Madison, NE,Stanton, NE}},{340,{Morrill, NE,Scotts Bluff, NE}}}
{{341,{Atlantic, NJ,Cape May, NJ}},{342,{Burlington, NJ,Camden, NJ}}}
{{343,{Cumberland, NJ,Salem, NJ}},{344,{Monmouth, NJ,Ocean, NJ}}}
{{345,{Morris, NJ,Sussex, NJ}},{346,{Bernalillo, NM,Sandoval, NM}}}
{{347,{Chaves, NM,Eddy, NM}},{348,{Curry, NM,Roosevelt, NM}}}
{{349,{Guadalupe, NM,Quay, NM}},{350,{Lincoln, NM,Otero, NM}}}
{{351,{Mora, NM,San Miguel, NM}},{352,{Rio Arriba, NM,Santa Fe, NM}}}
{{353,{Albany, NY,Rensselaer, NY}},{354,{Broome, NY,Tioga, NY}}}
{{355,{Columbia, NY,Greene, NY}},{356,{Delaware, NY,Otsego, NY}}}
{{357,{Erie, NY,Niagara, NY}},{358,{Fulton, NY,Montgomery, NY}}}
{{359,{Genesee, NY,Wyoming, NY}},{360,{Monroe, NY,Wayne, NY}}}
{{361,{Onondaga, NY,Oswego, NY}},{362,{Saratoga, NY,Schenectady, NY}}}
{{363,{Warren, NY,Washington, NY}},{364,{Alamance, NC,Caswell, NC}}}
{{365,{Beaufort, NC,Pitt, NC}},{366,{Bertie, NC,Hertford, NC}}}
{{367,{Bladen, NC,Columbus, NC}},{368,{Buncombe, NC,Henderson, NC}}}
{{369,{Burke, NC,Caldwell, NC}},{370,{Cabarrus, NC,Rowan, NC}}}
{{371,{Carteret, NC,Craven, NC}},{372,{Chowan, NC,Gates, NC}}}
{{373,{Cleveland, NC,Gaston, NC}},{374,{Currituck, NC,Dare, NC}}}
{{375,{Durham, NC,Orange, NC}},{376,{Edgecombe, NC,Nash, NC}}}
{{377,{Greene, NC,Wilson, NC}},{378,{Guilford, NC,Randolph, NC}}}
{{379,{Halifax, NC,Northampton, NC}},{380,{Haywood, NC,Madison, NC}}}
{{381,{Jackson, NC,Swain, NC}},{382,{Johnston, NC,Wake, NC}}}
{{383,{Mecklenburg, NC,Union, NC}},{384,{Montgomery, NC,Stanly, NC}}}
{{385,{Polk, NC,Rutherford, NC}},{386,{Barnes, ND,Griggs, ND}}}
{{387,{Benson, ND,Ramsey, ND}},{388,{Burleigh, ND,Morton, ND}}}
{{389,{Dickey, ND,LaMoure, ND}},{390,{Dunn, ND,Stark, ND}}}
{{391,{Foster, ND,Stutsman, ND}},{392,{Logan, ND,McIntosh, ND}}}
{{393,{McKenzie, ND,Mountrail, ND}},{394,{McLean, ND,Mercer, ND}}}
{{395,{Pembina, ND,Walsh, ND}},{396,{Ransom, ND,Sargent, ND}}}
{{397,{Steele, ND,Traill, ND}},{398,{Allen, OH,Auglaize, OH}}}
{{399,{Athens, OH,Hocking, OH}},{400,{Belmont, OH,Jefferson, OH}}}
{{401,{Butler, OH,Hamilton, OH}},{402,{Champaign, OH,Clark, OH}}}
{{403,{Clinton, OH,Highland, OH}},{404,{Crawford, OH,Richland, OH}}}
{{405,{Cuyahoga, OH,Lorain, OH}},{406,{Defiance, OH,Williams, OH}}}
{{407,{Erie, OH,Huron, OH}},{408,{Fulton, OH,Henry, OH}}}
{{409,{Greene, OH,Montgomery, OH}},{410,{Guernsey, OH,Noble, OH}}}
{{411,{Hardin, OH,Logan, OH}},{412,{Jackson, OH,Vinton, OH}}}
{{413,{Lucas, OH,Wood, OH}},{414,{Mahoning, OH,Trumbull, OH}}}
{{415,{Marion, OH,Morrow, OH}},{416,{Mercer, OH,Van Wert, OH}}}
{{417,{Miami, OH,Shelby, OH}},{418,{Muskingum, OH,Perry, OH}}}
{{419,{Ottawa, OH,Sandusky, OH}},{420,{Pickaway, OH,Ross, OH}}}
{{421,{Pike, OH,Scioto, OH}},{422,{Portage, OH,Summit, OH}}}
{{423,{Alfalfa, OK,Woods, OK}},{424,{Atoka, OK,Coal, OK}}}
{{425,{Beckham, OK,Roger Mills, OK}},{426,{Blaine, OK,Major, OK}}}
{{427,{Carter, OK,Love, OK}},{428,{Cherokee, OK,Muskogee, OK}}}
{{429,{Cleveland, OK,Oklahoma, OK}},{430,{Custer, OK,Washita, OK}}}
{{431,{Delaware, OK,Ottawa, OK}},{432,{Jackson, OK,Kiowa, OK}}}
{{433,{Johnston, OK,Marshall, OK}},{434,{Kay, OK,Osage, OK}}}
{{435,{Kingfisher, OK,Logan, OK}},{436,{Nowata, OK,Washington, OK}}}
{{437,{Baker, OR,Union, OR}},{438,{Benton, OR,Linn, OR}}}
{{439,{Clackamas, OR,Multnomah, OR}},{440,{Clatsop, OR,Columbia, OR}}}
{{441,{Jackson, OR,Josephine, OR}},{442,{Marion, OR,Polk, OR}}}
{{443,{Adams, PA,York, PA}},{444,{Allegheny, PA,Westmoreland, PA}}}
{{445,{Cambria, PA,Somerset, PA}},{446,{Carbon, PA,Monroe, PA}}}
{{447,{Clinton, PA,Lycoming, PA}},{448,{Crawford, PA,Erie, PA}}}
{{449,{Cumberland, PA,Dauphin, PA}},{450,{Fayette, PA,Greene, PA}}}
{{451,{Huntingdon, PA,Mifflin, PA}},{452,{Juniata, PA,Perry, PA}}}
{{453,{Lehigh, PA,Northampton, PA}},{454,{Montour, PA,Northumberland, PA}}}
{{455,{Susquehanna, PA,Wyoming, PA}},{456,{Bristol, RI,Newport, RI}}}
{{457,{Kent, RI,Providence, RI}},{458,{Aiken, SC,Edgefield, SC}}}
{{459,{Beaufort, SC,Jasper, SC}},{460,{Berkeley, SC,Charleston, SC}}}
{{461,{Calhoun, SC,Orangeburg, SC}},{462,{Clarendon, SC,Sumter, SC}}}

{{463,{Darlington, SC,Florence, SC}},{464,{Dillon, SC,Marion, SC}}}
{{465,{Georgetown, SC,Horry, SC}},{466,{Lexington, SC,Richland, SC}}}
{{467,{Newberry, SC,Saluda, SC}},{468,{Bon Homme, SD,Yankton, SD}}}
{{469,{Brule, SD,Lyman, SD}},{470,{Charles Mix, SD,Douglas, SD}}}
{{471,{Clay, SD,Union, SD}},{472,{Custer, SD,Fall River, SD}}}
{{473,{Davison, SD,Hanson, SD}},{474,{Day, SD,Marshall, SD}}}
{{475,{Dewey, SD,Ziebach, SD}},{476,{Grant, SD,Roberts, SD}}}
{{477,{Gregory, SD,Tripp, SD}},{478,{Hughes, SD,Stanley, SD}}}
{{479,{Lake, SD,Moody, SD}},{480,{Lincoln, SD,Minnehaha, SD}}}
{{481,{Meade, SD,Pennington, SD}},{482,{Mellette, SD,Todd, SD}}}
{{483,{Bradley, TN,Polk, TN}},{484,{Carter, TN,Washington, TN}}}
{{485,{Coffee, TN,Franklin, TN}},{486,{Cumberland, TN,Fentress, TN}}}
{{487,{Davidson, TN,Rutherford, TN}},{488,{Decatur, TN,Henderson, TN}}}
{{489,{Fayette, TN,Hardeman, TN}},{490,{Grainger, TN,Union, TN}}}
{{491,{Grundy, TN,Marion, TN}},{492,{Hardin, TN,McNairy, TN}}}
{{493,{Houston, TN,Stewart, TN}},{494,{Jackson, TN,Smith, TN}}}
{{495,{Lewis, TN,Perry, TN}},{496,{Morgan, TN,Roane, TN}}}
{{497,{Obion, TN,Weakley, TN}},{498,{Overton, TN,Putnam, TN}}}
{{499,{Robertson, TN,Sumner, TN}},{500,{Angelina, TX,Nacogdoches, TX}}}
{{501,{Bandera, TX,Kendall, TX}},{502,{Bell, TX,Coryell, TX}}}
{{503,{Brazoria, TX,Galveston, TX}},{504,{Brown, TX,Coleman, TX}}}
{{505,{Burnet, TX,Llano, TX}},{506,{Cameron, TX,Hidalgo, TX}}}
{{507,{Carson, TX,Gray, TX}},{508,{Cass, TX,Morris, TX}}}
{{509,{Cherokee, TX,Smith, TX}},{510,{Colorado, TX,Fayette, TX}}}
{{511,{Comanche, TX,Erath, TX}},{512,{Cooke, TX,Montague, TX}}}
{{513,{Culberson, TX,Hudspeth, TX}},{514,{Dallam, TX,Hartley, TX}}}
{{515,{DeWitt, TX,Lavaca, TX}},{516,{Duval, TX,Jim Wells, TX}}}
{{517,{Ector, TX,Midland, TX}},{518,{Edwards, TX,Real, TX}}}
{{519,{Ellis, TX,Navarro, TX}},{520,{Falls, TX,McLennan, TX}}}
{{521,{Fisher, TX,Nolan, TX}},{522,{Fort Bend, TX,Harris, TX}}}
{{523,{Gaines, TX,Terry, TX}},{524,{Gillespie, TX,Kerr, TX}}}
{{525,{Hardeman, TX,Wilbarger, TX}},{526,{Hardin, TX,Tyler, TX}}}
{{527,{Haskell, TX,Knox, TX}},{528,{Hopkins, TX,Wood, TX}}}
{{529,{Jasper, TX,Newton, TX}},{530,{Jefferson, TX,Orange, TX}}}
{{531,{Lamar, TX,Red River, TX}},{532,{Lipscomb, TX,Ochiltree, TX}}}
{{533,{Moore, TX,Sherman, TX}},{534,{Nueces, TX,San Patricio, TX}}}
{{535,{Potter, TX,Randall, TX}},{536,{Runnels, TX,Tom Green, TX}}}
{{537,{Sabine, TX,San Augustine, TX}},{538,{Shackelford, TX,Throckmorton, TX}}}
{{539,{Travis, TX,Williamson, TX}},{540,{Box Elder, UT,Cache, UT}}}
{{541,{Carbon, UT,Emery, UT}},{542,{Davis, UT,Weber, UT}}}
{{543,{Duchesne, UT,Uintah, UT}},{544,{Garfield, UT,Kane, UT}}}
{{545,{Iron, UT,Washington, UT}},{546,{Juab, UT,Millard, UT}}}
{{547,{Salt Lake, UT,Utah, UT}},{548,{Sanpete, UT,Sevier, UT}}}
{{549,{Summit, UT,Wasatch, UT}},{550,{Addison, VT,Rutland, VT}}}
{{551,{Caledonia, VT,Orleans, VT}},{552,{Chittenden, VT,Franklin, VT}}}
{{553,{Orange, VT,Washington, VT}},{554,{Accomack, VA,Northampton, VA}}}
{{555,{Albemarle, VA,Greene, VA}},{556,{Alleghany, VA,Bath, VA}}}
{{557,{Augusta, VA,Rockingham, VA}},{558,{Carroll, VA,Grayson, VA}}}
{{559,{Charles City, VA,New Kent, VA}},{560,{Charlotte, VA,Lunenburg, VA}}}
{{561,{Chesterfield, VA,Henrico, VA}},{562,{Cumberland, VA,Prince Edward, VA}}}
{{563,{Dinwiddie, VA,Prince George, VA}},{564,{Essex, VA,Richmond, VA}}}
{{565,{Gloucester, VA,Mathews, VA}},{566,{Goochland, VA,Louisa, VA}}}
{{567,{James City, VA,York, VA}},{568,{King George, VA,Westmoreland, VA}}}
{{569,{Montgomery, VA,Pulaski, VA}},{570,{Shenandoah, VA,Warren, VA}}}
{{571,{Chesapeake, VA,Virginia Beach, VA}},{572,{Hampton, VA,Newport News, VA}}}
{{573,{Adams, WA,Grant, WA}},{574,{Benton, WA,Franklin, WA}}}
{{575,{Chelan, WA,Douglas, WA}},{576,{Clallam, WA,Jefferson, WA}}}
{{577,{Clark, WA,Cowlitz, WA}},{578,{Ferry, WA,Okanogan, WA}}}
{{579,{Grays Harbor, WA,Pacific, WA}},{580,{King, WA,Snohomish, WA}}}
{{581,{Kitsap, WA,Mason, WA}},{582,{Kittitas, WA,Yakima, WA}}}
{{583,{Lewis, WA,Thurston, WA}},{584,{Skagit, WA,Whatcom, WA}}}
{{585,{Spokane, WA,Stevens, WA}},{586,{Barbour, WV,Randolph, WV}}}
{{587,{Berkeley, WV,Jefferson, WV}},{588,{Brooke, WV,Hancock, WV}}}
{{589,{Cabell, WV,Wayne, WV}},{590,{Fayette, WV,Raleigh, WV}}}
{{591,{Grant, WV,Hardy, WV}},{592,{Kanawha, WV,Putnam, WV}}}

{{593,{Lewis, WV,Upshur, WV}},{594,{Marshall, WV,Ohio, WV}}}
{{595,{Nicholas, WV,Webster, WV}},{596,{Pleasants, WV,Ritchie, WV}}}
{{597,{Tyler, WV,Wetzel, WV}},{598,{Ashland, WI,Bayfield, WI}}}
{{599,{Brown, WI,Oconto, WI}},{600,{Chippewa, WI,Eau Claire, WI}}}
{{601,{Clark, WI,Taylor, WI}},{602,{Door, WI,Kewaunee, WI}}}
{{603,{Forest, WI,Langlade, WI}},{604,{Grant, WI,Iowa, WI}}}
{{605,{Green, WI,Lafayette, WI}},{606,{Jackson, WI,Trempealeau, WI}}}
{{607,{Juneau, WI,Monroe, WI}},{608,{Kenosha, WI,Racine, WI}}}
{{609,{La Crosse, WI,Vernon, WI}},{610,{Lincoln, WI,Marathon, WI}}}
{{611,{Manitowoc, WI,Sheboygan, WI}},{612,{Milwaukee, WI,Waukesha, WI}}}
{{613,{Oneida, WI,Vilas, WI}},{614,{Outagamie, WI,Winnebago, WI}}}
{{615,{Ozaukee, WI,Washington, WI}},{616,{Portage, WI,Wood, WI}}}
{{617,{Price, WI,Rusk, WI}},{618,{Shawano, WI,Waupaca, WI}}}
{{619,{Albany, WY,Laramie, WY}},{620,{Big Horn, WY,Park, WY}}}
{{621,{Goshen, WY,Platte, WY}},{622,{Johnson, WY,Sheridan, WY}}}
{623,{Sweetwater, WY,Uinta, WY}}

**C. Isolated Counties having 1 in both corresponding row and column**

{{1,Crenshaw, AL},{2,Pike, AL},{3,Bullock, AL},{4,Macon, AL}}
{{5,Bibb, AL},{6,Chilton, AL},{7,Randolph, GA},{8,Quitman, GA}}
{{9,Barbour, AL},{10,Sumter, AL},{11,Greene, AL},{12,Marengo, AL}}
{{13,Hale, AL},{14,Perry, AL},{15,Dallas, AL},{16,Lowndes, AL}}
{{17,Butler, AL},{18,Troup, GA},{19,Floyd, GA},{20,Wilcox, AL}}
{{21,Clarke, AL},{22,Douglas, GA},{23,Carroll, GA},{24,Haralson, GA}}
{{25,Cleburne, AL},{26,Clay, AL},{27,Fayette, AL},{28,Henry, AL}}
{{29,Lamar, AL},{30,Pickens, AL},{31,Randolph, AL},{32,Adams, ID}}
{{33,Washington, ID},{34,Clearwater, ID},{35,Benewah, ID},{36,Shoshone, ID}}
{{37,Dillingham, AK},{38,Kodiak Island, AK},{39,Sitka, AK},{40,Skagway-Hoonah-Angoon, AK}}
{{41,Wrangell-Petersburg, AK},{42,Northwest Arctic, AK},{43,McCone, MT},{44,Meagher, MT}}
{{45,Broadwater, MT},{46,Wallowa, OR},{47,Cochise, AZ},{48,Pima, AZ}}
{{49,Maricopa, AZ},{50,Pinal, AZ},{51,Gila, AZ},{52,La Paz, AZ}}
{{53,Imperial, CA},{54,Ashley, AR},{55,Bradley, AR},{56,Carroll, AR}}
{{57,Yalobusha, MS},{58,Yazoo, MS},{59,Humphreys, MS},{60,Issaquena, MS}}
{{61,Sharkey, MS},{62,Tate, MS},{63,Panola, MS},{64,Quitman, MS}}
{{65,Tallahatchie, MS},{66,Coahoma, MS},{67,Bolivar, MS},{68,Sunflower, MS}}
{{69,Washington, MS},{70,Chicot, AR},{71,Desha, AR},{72,Drew, AR}}
{{73,Lincoln, AR},{74,Jefferson, AR},{75,Grant, AR},{76,Clark, AR}}
{{77,White, AR},{78,Cleburne, AR},{79,Pittsburg, OK},{80,Haskell, OK}}
{{81,Le Flore, OK},{82,Sequoyah, OK},{83,Adair, OK},{84,McDonald, MO}}
{{85,Lafayette, AR},{86,Columbia, AR},{87,St. Francis, AR},{88,Crittenden, AR}}
{{89,Polk, AR},{90,Scott, AR},{91,Logan, AR},{92,Franklin, AR}}
{{93,Sevier, AR},{94,Richland, IL},{95,Johnson, IL},{96,Union, IL}}
{{97,Alexander, IL},{98,Pulaski, IL},{99,Mississippi, MO},{100,New Madrid, MO}}
{{101,Dunklin, MO},{102,Pemiscot, MO},{103,Union, AR},{104,Ouachita, AR}}
{{105,Phillips, AR},{106,Monroe, AR},{107,San Mateo, CA},{108,Santa Clara, CA}}
{{109,Alameda, CA},{110,Camas, ID},{111,Contra Costa, CA},{112,Sumter, FL}}
{{113,Page, VA},{114,Del Norte, CA},{115,Trinity, CA},{116,Tuolumne, CA}}
{{117,Mariposa, CA},{118,Stanislaus, CA},{119,Solano, CA},{120,Riverside, CA}}
{{121,Santa Barbara, CA},{122,Huerfano, CO},{123,Las Animas, CO},{124,Cibola, NM}}
{{125,Catron, NM},{126,Jackson, CO},{127,Grand, CO},{128,Gunnison, CO}}
{{129,Lake, CO},{130,Lincoln, MT},{131,Flathead, MT},{132,Lake, MT}}
{{133,Sanders, MT},{134,Sheridan, MT},{135,Valley, MT},{136,Roosevelt, MT}}
{{137,Summit, CO},{138,Park, CO},{139,Teller, CO},{140,El Paso, CO}}
{{141,Fremont, CO},{142,Custer, CO},{143,Gilpin, CO},{144,Clear Creek, CO}}
{{145,Costilla, CO},{146,Crowley, CO},{147,Pitkin, CO},{148,Eagle, CO}}
{{149,Elbert, CO},{150,Garfield, CO},{151,Cheyenne, KS},{152,Sherman, KS}}
{{153,Kit Carson, CO},{154,Otero, CO},{155,Pueblo, CO},{156,Logan, CO}}
{{157,Woodward, OK},{158,Ellis, OK},{159,Grant, OK},{160,Garfield, OK}}
{{161,Payne, OK},{162,Noble, OK},{163,Pawnee, OK},{164,Rio Blanco, CO}}
{{165,Bronx, NY},{166,Westchester, NY},{167,Fairfield, CT},{168,New Haven, CT}}
{{169,Cecil, MD},{170,Hernando, FL},{171,Citrus, FL},{172,Marion, FL}}
{{173,Alachua, FL},{174,Putnam, FL},{175,Bradford, FL},{176,Broward, FL}}

{{177,Leon, FL},{178,Wakulla, FL},{179,Jefferson, FL},{180,Madison, FL}}
{{181,Lafayette, FL},{182,Taylor, FL},{183,Flagler, FL},{184,Franklin, FL}}
{{185,Gulf, FL},{186,Hamilton, FL},{187,Palm Beach, FL},{188,Martin, FL}}
{{189,Bledsoe, TN},{190,Rhea, TN},{191,Union, FL},{192,DeKalb, GA}}
{{193,Gwinnett, GA},{194,Walton, GA},{195,Ware, GA},{196,Pierce, GA}}
{{197,Bacon, GA},{198,Jeff Davis, GA},{199,Jackson, GA},{200,Hall, GA}}
{{201,White, GA},{202,Habersham, GA},{203,Banks, GA},{204,Tift, GA}}
{{205,Berrien, GA},{206,Dodge, GA},{207,Oconee, SC},{208,Stephens, GA}}
{{209,Franklin, GA},{210,Hart, GA},{211,Elbert, GA},{212,Wayne, GA}}
{{213,McIntosh, GA},{214,Glynn, GA},{215,Bulloch, GA},{216,Henry, GA}}
{{217,Butts, GA},{218,Camden, GA},{219,Screven, GA},{220,Candler, GA}}
{{221,Chattooga, GA},{222,Cherokee, GA},{223,Cook, GA},{224,Colquitt, GA}}
{{225,Monroe, GA},{226,Crawford, GA},{227,Dade, GA},{228,Dawson, GA}}
{{229,Emanuel, GA},{230,Pickens, GA},{231,Gilmer, GA},{232,Fannin, GA}}
{{233,Putnam, GA},{234,Morgan, GA},{235,Greene, GA},{236,Taliaferro, GA}}
{{237,Glascock, GA},{238,Lumpkin, GA},{239,Jefferson, GA},{240,Chase, KS}}
{{241,Morris, KS},{242,Dickinson, KS},{243,Geary, KS},{244,Liberty, GA}}
{{245,Long, GA},{246,Taylor, GA},{247,Clay, NC},{248,Douglas, NV}}
{{249,Carson City, NV},{250,Washoe, NV},{251,Lyon, NV},{252,Churchill, NV}}
{{253,Mineral, NV},{254,Lander, NV},{255,Lincoln, WA},{256,Garfield, WA}}
{{257,Columbia, WA},{258,Walla Walla, WA},{259,Umatilla, OR},{260,Morrow, OR}}
{{261,Gilliam, OR},{262,Wheeler, OR},{263,Grant, OR},{264,Harney, OR}}
{{265,Hood River, OR},{266,Wasco, OR},{267,Klickitat, WA},{268,Skamania, WA}}
{{269,Bear Lake, ID},{270,Caribou, ID},{271,Oneida, ID},{272,Clark, ID}}
{{273,Lemhi, ID},{274,Lewis, MO},{275,Adams, IL},{276,Bond, IL}}
{{277,Brown, IL},{278,LaSalle, IL},{279,Bureau, IL},{280,Pike, IL}}
{{281,Champaign, IL},{282,Piatt, IL},{283,Douglas, IL},{284,Edwards, IL}}
{{285,Jasper, IL},{286,Fulton, IL},{287,Grundy, IL},{288,McDonough, IL}}
{{289,Henderson, IL},{290,Wayne, MO},{291,Stoddard, MO},{292,Butler, MO}}
{{293,Ripley, MO},{294,Livingston, IL},{295,Moultrie, IL},{296,Macon, IL}}
{{297,Logan, IL},{298,McHenry, IL},{299,McLean, IL},{300,Woodford, IL}}
{{301,Marshall, IL},{302,Mason, IL},{303,Massac, IL},{304,Pope, IL}}
{{305,Randolph, IL},{306,Morgan, IL},{307,Rush, IN},{308,Decatur, IN}}
{{309,Bartholomew, IN},{310,Dawson, MT},{311,Fallon, MT},{312,Custer, MT}}
{{313,Rosebud, MT},{314,Big Horn, MT},{315,Yellowstone, MT},{316,Carbon, MT}}
{{317,Stillwater, MT},{318,Sweet Grass, MT},{319,Wheatland, MT},{320,Tipton, IN}}
{{321,Howard, IN},{322,Miami, IN},{323,Marion, IN},{324,Jennings, IN}}
{{325,Whitley, IN},{326,Owen, IN},{327,Monroe, IN},{328,Lawrence, IN}}
{{329,Starke, IN},{330,Orange, IN},{331,Linn, IA},{332,Hamilton, IA}}
{{333,Webster, IA},{334,Calhoun, IA},{335,Greene, IA},{336,Boone, IA}}
{{337,Harrison, IA},{338,Crawford, IA},{339,Des Moines, IA},{340,Henry, IA}}
{{341,Washington, IA},{342,Keokuk, IA},{343,Iowa, IA},{344,Cedar, IA}}
{{345,Woodbury, IA},{346,Plymouth, IA},{347,Cherokee, IA},{348,Jones, IA}}
{{349,Delaware, IA},{350,Clayton, IA},{351,Story, IA},{352,Polk, IA}}
{{353,Mercer, MO},{354,Harrison, MO},{355,Gentry, MO},{356,Worth, MO}}
{{357,Ringgold, IA},{358,Union, IA},{359,Deer Lodge, MT},{360,Silver Bow, MT}}
{{361,Powell, MT},{362,Toole, MT},{363,Glacier, MT},{364,Cascade, MT}}
{{365,Chouteau, MT},{366,Liberty, MT},{367,Powder River, MT},{368,Carter, MT}}
{{369,Monona, IA},{370,Knox, OH},{371,Bourbon, KS},{372,Allen, KS}}
{{373,Jefferson, KS},{374,Atchison, KS},{375,Russell, KS},{376,Ellis, KS}}
{{377,Rush, KS},{378,Barber, KS},{379,Doniphan, KS},{380,Brown, KS}}
{{381,Zavala, TX},{382,Uvalde, TX},{383,Maverick, TX},{384,Val Verde, TX}}
{{385,Kinney, TX},{386,Decatur, KS},{387,Rawlins, KS},{388,Washington, KS}}
{{389,Marshall, KS},{390,Nemaha, KS},{391,Jackson, KS},{392,Wabaunsee, KS}}
{{393,Polk, TX},{394,Comanche, KS},{395,Texas, OK},{396,Seward, KS}}
{{397,Finney, KS},{398,Ford, KS},{399,Montgomery, KS},{400,Norton, KS}}
{{401,Graham, KS},{402,Socorro, NM},{403,Los Alamos, NM},{404,Stevens, KS}}
{{405,Grant, KS},{406,Gray, KS},{407,Greenwood, KS},{408,Harper, KS}}
{{409,Meade, KS},{410,Haskell, KS},{411,Stanton, KS},{412,Kiowa, KS}}
{{413,Neosho, KS},{414,Smith, KS},{415,Scott, KS},{416,Todd, KY}}
{{417,Logan, KY},{418,Warren, KY},{419,Allen, KY},{420,Isle of Wight, VA}}
{{421,Southampton, VA},{422,Colonial Heights, VA},{423,Ballard, KY},{424,Bracken, KY}}
{{425,Lake, MI},{426,Wolfe, KY},{427,Hardin, KY},{428,Meade, KY}}
{{429,Breckinridge, KY},{430,Edmonson, KY},{431,Butler, KY},{432,Carlisle, KY}}

{{433,Pike, KY},{434,Floyd, KY},{435,Hickman, KY},{436,Henry, KY}}
{{437,Shelby, KY},{438,Spencer, KY},{439,Pendleton, KY},{440,Grant, KY}}
{{441,Owen, KY},{442,Madison, KY},{443,Rockcastle, KY},{444,Simpson, KY}}
{{445,Allen, LA},{446,Jefferson Davis, LA},{447,Calcasieu, LA},{448,Beauregard, LA}}
{{449,Vernon, LA},{450,Washington, LA},{451,Pearl River, MS},{452,Hancock, MS}}
{{453,St. Bernard, LA},{454,Plaquemines, LA},{455,West Feliciana, LA},{456,East Feliciana, LA}}
{{457,Evangeline, LA},{458,St. Landry, LA},{459,Acadia, LA},{460,Vermilion, LA}}
{{461,Iberia, LA},{462,Iberville, LA},{463,West Baton Rouge, LA},{464,Pointe Coupee, LA}}
{{465,Avoyelles, LA},{466,Morehouse, LA},{467,Ouachita, LA},{468,Union, LA}}
{{469,Lincoln, LA},{470,Jackson, LA},{471,Catahoula, LA},{472,La Salle, LA}}
{{473,Caldwell, LA},{474,Natchitoches, LA},{475,Sabine, LA},{476,De Soto, LA}}
{{477,East Baton Rouge, LA},{478,Tangipahoa, LA},{479,St. Helena, LA},{480,Perry, MS}}
{{481,Greene, MS},{482,George, MS},{483,Winn, LA},{484,Allegany, MD}}
{{485,St. Mary's, MD},{486,Howard, MD},{487,Prince George's, MD},{488,Montgomery, MD}}
{{489,Monongalia, WV},{490,Preston, WV},{491,Garrett, MD},{492,Washington, MD}}
{{493,Barnstable, MA},{494,Plymouth, MA},{495,Dukes, MA},{496,Middlesex, MA}}
{{497,Essex, MA},{498,Nantucket, MA},{499,Emmet, MI},{500,Charlevoix, MI}}
{{501,Antrim, MI},{502,Manistee, MI},{503,Mason, MI},{504,Keweenaw, MI}}
{{505,Ontonagon, MI},{506,Baraga, MI},{507,Barry, MI},{508,Calhoun, MI}}
{{509,Jackson, MI},{510,Lenawee, MI},{511,Hillsdale, MI},{512,Branch, MI}}
{{513,Gladwin, MI},{514,Shiawassee, MI},{515,Crawford, MI},{516,Houghton, MI}}
{{517,Oakland, MI},{518,Macomb, MI},{519,St. Clair, MI},{520,Kittson, MN}}
{{521,Red Lake, MN},{522,Clearwater, MN},{523,Beltrami, MN},{524,Chippewa, MN}}
{{525,Hubbard, MN},{526,Lac qui Parle, MN},{527,Scott, MN},{528,Le Sueur, MN}}
{{529,Pipestone, MN},{530,Rock, MN},{531,Nobles, MN},{532,Murray, MN}}
{{533,Morrison, MN},{534,Sibley, MN},{535,Renville, MN},{536,St. Louis, MN}}
{{537,Scott, MS},{538,Newton, MS},{539,Neshoba, MS},{540,Winston, MS}}
{{541,Calhoun, MS},{542,Chickasaw, MS},{543,Oktibbeha, MS},{544,Copiah, MS}}
{{545,Lincoln, MS},{546,Lawrence, MS},{547,Jefferson Davis, MS},{548,Hinds, MS}}
{{549,Union, MS},{550,Audrain, MO},{551,Bates, MO},{552,Monroe, MO}}
{{553,Shelby, MO},{554,Macon, MO},{555,Randolph, MO},{556,Douglas, MO}}
{{557,Ozark, MO},{558,Howell, MO},{559,Oregon, MO},{560,Shannon, MO}}
{{561,Carter, MO},{562,Franklin, MO},{563,Crawford, MO},{564,Pulaski, MO}}
{{565,Laclede, MO},{566,Phelps, MO},{567,St. Louis, MO},{568,St. Charles, MO}}
{{569,Lincoln, MO},{570,Warren, MO},{571,Montgomery, MO},{572,St. Clair, MO}}
{{573,Saline, MO},{574,Lafayette, MO},{575,Reynolds, MO},{576,Madison, MO}}
{{577,Perry, MO},{578,Ste. Genevieve, MO},{579,Pocahontas, WV},{580,Pendleton, WV}}
{{581,Fairfax, VA},{582,Prince William, VA},{583,Stafford, VA},{584,Spotsylvania, VA}}
{{585,Caroline, VA},{586,Pend Oreille, WA},{587,San Juan, WA},{588,Phillips, MT}}
{{589,Washakie, WY},{590,Weston, WY},{591,Crook, WY},{592,Butte, SD}}
{{593,Lawrence, SD},{594,Campbell, WY},{595,Converse, WY},{596,Natrona, WY}}
{{597,Fremont, WY},{598,Carbon, WY},{599,Prairie, MT},{600,Holt, NE}}
{{601,Antelope, NE},{602,Thomas, NE},{603,Dawes, NE},{604,Box Butte, NE}}
{{605,Chase, NE},{606,Perkins, NE},{607,Keith, NE},{608,Lincoln, NE}}
{{609,Custer, NE},{610,Dawson, NE},{611,Buffalo, NE},{612,Garden, NE}}
{{613,Grant, NE},{614,Kearney, NE},{615,Phelps, NE},{616,Harlan, NE}}
{{617,Furnas, NE},{618,Gosper, NE},{619,Rock, NE},{620,Nuckolls, NE}}
{{621,Sublette, WY},{622,Niobrara, WY},{623,Elko, NV},{624,Nye, NV}}
{{625,White Pine, NV},{626,Eureka, NV},{627,Humboldt, NV},{628,Pershing, NV}}
{{629,Rockingham, NH},{630,Hillsborough, NH},{631,Merrimack, NH},{632,Windsor, VT}}
{{633,Bergen, NJ},{634,Union, NJ},{635,Middlesex, NJ},{636,Somerset, NJ}}
{{637,Hunterdon, NJ},{638,Harding, NM},{639,Crane, TX},{640,Yoakum, TX}}
{{641,Cattaraugus, NY},{642,Chautauqua, NY},{643,Steuben, NY},{644,Chemung, NY}}
{{645,Clinton, NY},{646,Tompkins, NY},{647,Cortland, NY},{648,Dutchess, NY}}
{{649,Essex, NY},{650,Franklin, NY},{651,St. Lawrence, NY},{652,Jefferson, NY}}
{{653,Queens, NY},{654,Nassau, NY},{655,Orange, NY},{656,Yates, NY}}
{{657,Schuyler, NY},{658,Seneca, NY},{659,Harrison, WV},{660,Doddridge, WV}}
{{661,Schoharie, NY},{662,Catawba, NC},{663,Alexander, NC},{664,Mitchell, NC}}
{{665,McDowell, NC},{666,Avery, NC},{667,Watauga, NC},{668,Ashe, NC}}
{{669,Alleghany, NC},{670,Wilkes, NC},{671,Yadkin, NC},{672,Davie, NC}}

{{673,Anson, NC},{674,Lee, NC},{675,Harnett, NC},{676,Sampson, NC}}
{{677,Duplin, NC},{678,Forsyth, NC},{679,Granville, NC},{680,Tyrrell, NC}}
{{681,Washington, NC},{682,Martin, NC},{683,Wayne, NC},{684,Lenoir, NC}}
{{685,Chesterfield, SC},{686,Marlboro, SC},{687,Scotland, NC},{688,Richmond, NC}}
{{689,New Hanover, NC},{690,Stokes, NC},{691,Surry, NC},{692,Patrick, VA}}
{{693,Henry, VA},{694,Franklin, VA},{695,Roanoke, VA},{696,Botetourt, VA}}
{{697,Brunswick, VA},{698,Mecklenburg, VA},{699,Halifax, VA},{700,Vance, NC}}
{{701,Warren, NC},{702,Adams, ND},{703,Ward, ND},{704,McHenry, ND}}
{{705,Pierce, ND},{706,Rolette, ND},{707,Bottineau, ND},{708,Cavalier, ND}}
{{709,Grant, ND},{710,Sheridan, ND},{711,Sioux, ND},{712,Brown, OH}}
{{713,Geauga, OH},{714,Tuscarawas, OH},{715,Harrison, OH},{716,Carroll, OH}}
{{717,Wayne, OH},{718,Holmes, OH},{719,Franklin, OH},{720,Madison, OH}}
{{721,Morgan, OH},{722,Putnam, OH},{723,Delta, TX},{724,Fannin, TX}}
{{725,Grayson, TX},{726,Murray, OK},{727,Garvin, OK},{728,McClain, OK}}
{{729,Grady, OK},{730,Caddo, OK},{731,Comanche, OK},{732,Caldwell, TX}}
{{733,Gonzales, TX},{734,Bee, TX},{735,Live Oak, TX},{736,Scurry, TX}}
{{737,Blanco, TX},{738,Mason, TX},{739,Matagorda, TX},{740,Wharton, TX}}
{{741,Wichita, TX},{742,Clay, TX},{743,Jefferson, OK},{744,Stephens, OK}}
{{745,Tillman, OK},{746,Greer, OK},{747,Harmon, OK},{748,Hughes, OK}}
{{749,Curry, OR},{750,Coos, OR},{751,Douglas, OR},{752,Yamhill, OR}}
{{753,Lincoln, OR},{754,Beaver, PA},{755,Lawrence, PA},{756,Mercer, PA}}
{{757,Venango, PA},{758,Clarion, PA},{759,Armstrong, PA},{760,Franklin, PA}}
{{761,Fulton, PA},{762,Bedford, PA},{763,Elk, PA},{764,McKean, PA}}
{{765,Potter, PA},{766,Schuylkill, PA},{767,Blair, PA},{768,Bradford, PA}}
{{769,Montgomery, PA},{770,Chester, PA},{771,Wayne, PA},{772,Lackawanna, PA}}
{{773,Luzerne, PA},{774,Lancaster, PA},{775,Tioga, PA},{776,Union, PA}}
{{777,Abbeville, SC},{778,Hampton, SC},{779,Allendale, SC},{780,Barnwell, SC}}
{{781,Chester, SC},{782,Greenwood, SC},{783,Laurens, SC},{784,Union, SC}}
{{785,Lancaster, SC},{786,Kershaw, SC},{787,Lee, SC},{788,Jerauld, SD}}
{{789,Sanborn, SD},{790,Miner, SD},{791,Beadle, SD},{792,Shannon, SD}}
{{793,Bennett, SD},{794,Spink, SD},{795,Brown, SD},{796,Corson, SD}}
{{797,Deuel, SD},{798,Edmunds, SD},{799,Turner, SD},{800,Hutchinson, SD}}
{{801,Hyde, SD},{802,Claiborne, TN},{803,Campbell, TN},{804,Anderson, TN}}
{{805,Wythe, VA},{806,Smyth, VA},{807,Washington, VA},{808,Sullivan, TN}}
{{809,Hawkins, TN},{810,Wayne, TN},{811,Lawrence, TN},{812,Giles, TN}}
{{813,Maury, TN},{814,Marshall, TN},{815,Bedford, TN},{816,Knox, TN}}
{{817,Blount, TN},{818,Macon, TN},{819,Trousdale, TN},{820,Unicoi, TN}}
{{821,Johnson, TN},{822,Lake, TN},{823,Dyer, TN},{824,Lauderdale, TN}}
{{825,Haywood, TN},{826,Lincoln, TN},{827,Loudon, TN},{828,Monroe, TN}}
{{829,McMinn, TN},{830,Kleberg, TX},{831,La Salle, TX},{832,Frio, TX}}
{{833,Atascosa, TX},{834,Medina, TX},{835,Mitchell, TX},{836,Reeves, TX}}
{{837,Ward, TX},{838,Winkler, TX},{839,Karnes, TX},{840,Aransas, TX}}
{{841,Irion, TX},{842,Reagan, TX},{843,Upton, TX},{844,Donley, TX}}
{{845,Hall, TX},{846,Briscoe, TX},{847,Refugio, TX},{848,Robertson, TX}}
{{849,Brazos, TX},{850,Burleson, TX},{851,Grimes, TX},{852,Waller, TX}}
{{853,Austin, TX},{854,Bailey, TX},{855,Baylor, TX},{856,Dawson, TX}}
{{857,Lynn, TX},{858,Hill, TX},{859,Bosque, TX},{860,Brewster, TX}}
{{861,Jackson, TX},{862,Calhoun, TX},{863,Walker, TX},{864,Jones, TX}}
{{865,Taylor, TX},{866,Callahan, TX},{867,Oldham, TX},{868,Deaf Smith, TX}}
{{869,Castro, TX},{870,Chambers, TX},{871,Cottle, TX},{872,Childress, TX}}
{{873,Victoria, TX},{874,Goliad, TX},{875,Dallas, TX},{876,Collingsworth, TX}}
{{877,Comal, TX},{878,Lee, TX},{879,Milam, TX},{880,Kimble, TX}}
{{881,Sutton, TX},{882,McCulloch, TX},{883,Concho, TX},{884,Garza, TX}}
{{885,Dickens, TX},{886,Jack, TX},{887,Young, TX},{888,Stephens, TX}}
{{889,Swisher, TX},{890,Floyd, TX},{891,Somervell, TX},{892,Hood, TX}}
{{893,Houston, TX},{894,Madison, TX},{895,Leon, TX},{896,Freestone, TX}}
{{897,Glasscock, TX},{898,Shelby, TX},{899,Panola, TX},{900,Rusk, TX}}
{{901,Gregg, TX},{902,Hockley, TX},{903,Lubbock, TX},{904,Lampasas, TX}}
{{905,Mills, TX},{906,Wheeler, TX},{907,Hemphill, TX},{908,Presidio, TX}}
{{909,Jeff Davis, TX},{910,Stonewall, TX},{911,Liberty, TX},{912,Upshur, TX}}
{{913,Marion, TX},{914,Roberts, TX},{915,Lamoille, VT},{916,Middlesex, VA}}
{{917,Lancaster, VA},{918,Northumberland, VA},{919,Nottoway, VA},{920,Amelia, VA}}
{{921,Clarke, VA},{922,Culpeper, VA},{923,Lee, VA},{924,Wise, VA}}
{{925,Frederick, VA},{926,Giles, VA},{927,Greensville, VA},{928,King William, VA}}
{{929,Madison, VA},{930,Rockbridge, VA},{931,Monroe, WV},{932,Greenbrier, WV}}

{{933,Summers, WV},{934,Wyoming, WV},{935,McDowell, WV},{936,Mercer, WV}}
{{937,Tazewell, VA},{938,Sussex, VA},{939,Mineral, WV},{940,Hampshire, WV}}
{{941,Morgan, WV},{942,Clay, WV},{943,Braxton, WV},{944,Gilmer, WV}}
{{945,Calhoun, WV},{946,Roane, WV},{947,Jackson, WV},{948,Walworth, WI}}
{{949,Rock, WI},{950,Dane, WI},{951,Columbia, WI},{952,Marquette, WI}}
{{953,Douglas, WI},{954,Dunn, WI},{955,Pepin, WI},{956,Dodge, WI}}
{{957,Fond du Lac, WI},{958,Green Lake, WI},{959,St. Croix, WI}}

**D. Isolated Counties having a 1 in either corresponding row and column, but not both**

{{1,Covington, AL},{2,Autauga, AL},{3,Terrell, GA},{4,Choctaw, AL}}
{{5,Meriwether, GA},{6,Chambers, AL},{7,Polk, GA},{8,Cherokee, AL}}
{{9,Paulding, GA},{10,Marion, AL},{11,Houston, AL},{12,Tuscaloosa, AL}}
{{13,Washington, AL},{14,Walker, AL},{15,Winston, AL},{16,Valley, ID}}
{{17,Aleutians West, AK},{18,Lake and Peninsula, AK},{19,Bristol Bay, AK},{20,Kenai Peninsula, AK}}
{{21,Juneau, AK},{22,North Slope, AK},{23,Nome, AK},{24,Wahkiakum, WA}}
{{25,Yakutat, AK},{26,Santa Cruz, AZ},{27,Yavapai, AZ},{28,Coconino, AZ}}
{{29,Mohave, AZ},{30,Humboldt, CA},{31,Yuma, AZ},{32,Stone, MS}}
{{33,Cleveland, AR},{34,Lafayette, MS},{35,Lonoke, AR},{36,Latimer, OK}}
{{37,Lee, AR},{38,Cross, AR},{39,Montgomery, AR},{40,Izard, AR}}
{{41,Fulton, AR},{42,Johnson, AR},{43,Howard, AR},{44,Little River, AR}}
{{45,Madison, AR},{46,Lawrence, IL},{47,Mississippi, AR},{48,Pike, AR}}
{{49,Stone, AR},{50,San Francisco, CA},{51,Blaine, ID},{52,Alpine, CA}}
{{53,Lake, FL},{54,Colusa, CA},{55,Lake, CA},{56,Mendocino, CA}}
{{57,San Joaquin, CA},{58,Merced, CA},{59,Lake, OR},{60,Modoc, CA}}
{{61,Napa, CA},{62,Sierra, CA},{63,Nevada, CA},{64,San Bernardino, CA}}
{{65,San Diego, CA},{66,San Luis Obispo, CA},{67,Ventura, CA},{68,De Baca, NM}}
{{69,Baca, CO},{70,Archuleta, CO},{71,Bent, CO},{72,McKinley, NM}}
{{73,Chaffee, CO},{74,Boundary, ID},{75,Taos, NM},{76,Douglas, CO}}
{{77,Wallace, KS},{78,Lincoln, CO},{79,Mesa, CO},{80,Dewey, OK}}
{{81,Mineral, CO},{82,Morgan, CO},{83,Kiowa, CO},{84,Prowers, CO}}
{{85,Phillips, CO},{86,Sedgwick, CO},{87,New York, NY},{88,Middlesex, CT}}
{{89,Harford, MD},{90,New Castle, DE},{91,Pasco, FL},{92,Miami-Dade, FL}}
{{93,Gadsden, FL},{94,Dixie, FL},{95,Volusia, FL},{96,Sequatchie, TN}}
{{97,Monroe, FL},{98,Okeechobee, FL},{99,Osceola, FL},{100,Polk, FL}}
{{101,St. Lucie, FL},{102,Fulton, GA},{103,Appling, GA},{104,Barrow, GA}}
{{105,Turner, GA},{106,Telfair, GA},{107,Bleckley, GA},{108,Transylvania, NC}}
{{109,Brantley, GA},{110,Bryan, GA},{111,Clayton, GA},{112,Nassau, FL}}
{{113,Hamilton, TN},{114,Catoosa, GA},{115,Cobb, GA},{116,Forsyth, GA}}
{{117,Calhoun, GA},{118,Early, GA},{119,Echols, GA},{120,Evans, GA}}
{{121,Baldwin, GA},{122,Hancock, GA},{123,Heard, GA},{124,Jasper, GA}}
{{125,Johnson, GA},{126,Laurens, GA},{127,Clark, KS},{128,Macon, GA}}
{{129,Marion, GA},{130,Baker, GA},{131,Miller, GA},{132,Clay, GA}}
{{133,Mitchell, GA},{134,Talbot, GA},{135,Tattnall, GA},{136,Cherokee, NC}}
{{137,Towns, GA},{138,Union, GA},{139,Washington, GA},{140,Treutlen, GA}}
{{141,Wheeler, GA},{142,Pulaski, GA},{143,Wilcox, GA},{144,Twiggs, GA}}
{{145,Wilkinson, GA},{146,Worth, GA},{147,El Dorado, CA},{148,Butte, ID}}
{{149,Custer, ID},{150,Rich, UT},{151,Franklin, ID},{152,Clark, MO}}
{{153,Schuyler, IL},{154,DeKalb, IL},{155,Calhoun, IL},{156,Vermilion, IL}}
{{157,White, IL},{158,De Witt, IL},{159,Ford, IL},{160,Crawford, IL}}
{{161,Will, IL},{162,Hardin, IL},{163,Bollinger, MO},{164,Lake, IL}}
{{165,Monroe, IL},{166,Cass, IL},{167,Putnam, IL},{168,Scott, IL}}
{{169,Stark, IL},{170,Wabash, IL},{171,Shelby, IN},{172,Benton, IN}}
{{173,Brown, IN},{174,Daniels, MT},{175,Cass, IN},{176,Harrison, IN}}
{{177,Crawford, IN},{178,Johnson, IN},{179,Hamilton, IN},{180,Jackson, IN}}
{{181,Posey, IN},{182,Knox, IN},{183,Allen, IN},{184,Kosciusko, IN}}
{{185,Putnam, IN},{186,LaPorte, IN},{187,Marshall, IN},{188,Daviess, IN}}
{{189,Martin, IN},{190,Hendricks, IN},{191,Morgan, IN},{192,LaGrange, IN}}
{{193,Noble, IN},{194,Washington, IN},{195,Johnson, IA},{196,Benton, IA}}
{{197,Wright, IA},{198,Shelby, IA},{199,Carroll, IA},{200,Dakota, NE}}
{{201,Dallas, IA},{202,Ida, IA},{203,Grundy, MO},{204,Madison, IA}}
{{205,Granite, MT},{206,Montgomery, IA},{207,Licking, OH},{208,Douglas, KS}}
{{209,Rooks, KS},{210,Pawnee, KS},{211,Barton, KS},{212,Dimmit, TX}}
{{213,Clay, KS},{214,Wise, TX},{215,Hodgeman, KS},{216,Edwards, KS}}

{{217,Cimarron, OK},{218,Sheridan, KS},{219,Gove, KS},{220,Wilson, KS}}
{{221,Valencia, NM},{222,Woodson, KS},{223,Hamilton, KS},{224,Kearny, KS}}
{{225,Kingman, KS},{226,Labette, KS},{227,Ellsworth, KS},{228,Lincoln, KS}}
{{229,Mitchell, KS},{230,Trego, KS},{231,Ness, KS},{232,Phillips, KS}}
{{233,Osborne, KS},{234,Pratt, KS},{235,Lane, KS},{236,Wichita, KS}}
{{237,Trigg, KY},{238,Suffolk, VA},{239,Robertson, KY},{240,Newaygo, MI}}
{{241,Breathitt, KY},{242,Larue, KY},{243,Grayson, KY},{244,Mingo, WV}}
{{245,Fulton, KY},{246,Oldham, KY},{247,Gallatin, KY},{248,Hancock, KY}}
{{249,Estill, KY},{250,Jackson, KY},{251,Johnson, KY},{252,Mason, KY}}
{{253,Bienville, LA},{254,Cameron, LA},{255,Red River, LA},{256,Ascension, LA}}
{{257,Livingston, LA},{258,Tensas, LA},{259,Madison, LA},{260,St. Tammany, LA}}
{{261,St. James, LA},{262,East Carroll, LA},{263,West Carroll, LA},{264,Wayne, MS}}
{{265,Charles, MD},{266,Calvert, MD},{267,Anne Arundel, MD},{268,Carroll, MD}}
{{269,District of Columbia, DC},{270,Frederick, MD},{271,Marion, WV},{272,Somerset,
MD}}
{{273,Worcester, MA},{274,Norfolk, MA},{275,Bristol, MA},{276,Suffolk, MA}}
{{277,Cheboygan, MI},{278,Benzie, MI},{279,Allegan, MI},{280,Midland, MI}}
{{281,Clare, MI},{282,Livingston, MI},{283,Clinton, MI},{284,Roscommon, MI}}
{{285,Kalkaska, MI},{286,Wayne, MI},{287,Marquette, MI},{288,Oscoda, MI}}
{{289,St. Joseph, MI},{290,Sanilac, MI},{291,Burke, ND},{292,Yellow Medicine, MN}}
{{293,Anoka, MN},{294,Hennepin, MN},{295,Dakota, MN},{296,Lincoln, MN}}
{{297,Lyon, MN},{298,Faribault, MN},{299,Martin, MN},{300,Koochiching, MN}}
{{301,Carver, MN},{302,Redwood, MN},{303,Rice, MN},{304,Carlton, MN}}
{{305,Todd, MN},{306,Wadena, MN},{307,Ramsey, MN},{308,Washington, MN}}
{{309,Leake, MS},{310,Attala, MS},{311,Tunica, MS},{312,Lowndes, MS}}
{{313,Clay, MS},{314,Covington, MS},{315,Madison, MS},{316,Franklin, MS}}
{{317,Jefferson, MS},{318,Monroe, MS},{319,Kemper, MS},{320,Noxubee, MS}}
{{321,Rankin, MS},{322,Pontotoc, MS},{323,Tippah, MS},{324,Pike, MO}}
{{325,Cass, MO},{326,Boone, MO},{327,Hamilton, IL},{328,Jefferson, MO}}
{{329,Chattahoochee, GA},{330,Dallas, MO},{331,Dent, MO},{332,St. Louis City, MO}}
{{333,Gasconade, MO},{334,Henry, MO},{335,Washington, MO},{336,Iron, MO}}
{{337,Carroll, MO},{338,Johnson, MO},{339,St. Francois, MO},{340,Petroleum, MT}}
{{341,Garfield, MT},{342,Mineral, MT},{343,Golden Valley, MT},{344,Musselshell, MT}}
{{345,Arlington, VA},{346,Hot Springs, WY},{347,Richland, MT},{348,Treasure, MT}}
{{349,Boyd, NE},{350,Kimball, NE},{351,Arthur, NE},{352,Blaine, NE}}
{{353,Sheridan, NE},{354,Dundy, NE},{355,Banner, NE},{356,Cherry, NE}}
{{357,Deuel, NE},{358,Cheyenne, NE},{359,Pawnee, NE},{360,Johnson, NE}}
{{361,Brown, NE},{362,Keya Paha, NE},{363,Hooker, NE},{364,Loup, NE}}
{{365,Logan, NE},{366,McPherson, NE},{367,Jewell, KS},{368,Pierce, NE}}
{{369,Richardson, NE},{370,Saline, NE},{371,Lincoln, WY},{372,Sioux, NE}}
{{373,Thayer, NE},{374,Tooele, UT},{375,Lincoln, NV},{376,Esmeralda, NV}}
{{377,Clark, NV},{378,Storey, NV},{379,Belknap, NH},{380,Strafford, NH}}
{{381,Carroll, NH},{382,Grafton, NH},{383,Sullivan, NH},{384,Hudson, NJ}}
{{385,Essex, NJ},{386,Passaic, NJ},{387,Warren, NJ},{388,Union, NM}}
{{389,Colfax, NM},{390,Luna, NM},{391,Grant, NM},{392,Terrell, TX}}
{{393,Lea, NM},{394,Torrance, NM},{395,Sierra, NM},{396,Allegany, NY}}
{{397,Livingston, NY},{398,Chenango, NY},{399,Cayuga, NY},{400,Putnam, NY}}
{{401,Hamilton, NY},{402,Oneida, NY},{403,Herkimer, NY},{404,Lewis, NY}}
{{405,Kings, NY},{406,Rockland, NY},{407,Ontario, NY},{408,Orleans, NY}}
{{409,Taylor, WV},{410,Suffolk, NY},{411,Sullivan, NY},{412,Ulster, NY}}
{{413,Lincoln, NC},{414,Yancey, NC},{415,Chatham, NC},{416,Davidson, NC}}
{{417,Franklin, NC},{418,Graham, NC},{419,Hyde, NC},{420,Iredell, NC}}
{{421,Jones, NC},{422,Moore, NC},{423,Brunswick, NC},{424,Camden, NC}}
{{425,Pamlico, NC},{426,Perquimans, NC},{427,Pasquotank, NC},{428,Pender, NC}}
{{429,Person, NC},{430,Pittsylvania, VA},{431,Rockingham, NC},{432,Hettinger, ND}}
{{433,Slope, ND},{434,Billings, ND},{435,Williams, ND},{436,Harding, SD}}
{{437,Bowman, ND},{438,Perkins, SD},{439,Renville, ND},{440,Oliver, ND}}
{{441,Towner, ND},{442,Wells, ND},{443,Clermont, OH},{444,Adams, OH}}
{{445,Lake, OH},{446,Ashtabula, OH},{447,Stark, OH},{448,Columbiana, OH}}
{{449,Medina, OH},{450,Coshocton, OH},{451,Fairfield, OH},{452,Delaware, OH}}
{{453,Union, OH},{454,Fayette, OH},{455,Monroe, OH},{456,Paulding, OH}}
{{457,Hinsdale, CO},{458,Bryan, OK},{459,Cotton, OK},{460,Mayes, OK}}
{{461,Craig, OK},{462,Hays, TX},{463,Pontotoc, OK},{464,Okmulgee, OK}}
{{465,McIntosh, OK},{466,Okfuskee, OK},{467,Seminole, OK},{468,Pottawatomie, OK}}
{{469,Tulsa, OK},{470,Wagoner, OK},{471,Lane, OR},{472,Washington, OR}}

{{473,Sherman, OR},{474,Tillamook, OR},{475,Butler, PA},{476,Cameron, PA}}
{{477,Berks, PA},{478,Philadelphia, PA},{479,Bucks, PA},{480,Centre, PA}}
{{481,Delaware, PA},{482,Pike, PA},{483,Columbia, PA},{484,Indiana, PA}}
{{485,Clearfield, PA},{486,Jefferson, PA},{487,Lebanon, PA},{488,Snyder, PA}}
{{489,Warren, PA},{490,McCormick, SC},{491,Colleton, SC},{492,Bamberg, SC}}
{{493,Spartanburg, SC},{494,Cherokee, SC},{495,York, SC},{496,Fairfield, SC}}
{{497,Williamsburg, SC},{498,Buffalo, SD},{499,Aurora, SD},{500,Kingsbury, SD}}
{{501,Brookings, SD},{502,Clark, SD},{503,Faulk, SD},{504,Codington, SD}}
{{505,Hamlin, SD},{506,McCook, SD},{507,Hand, SD},{508,Jackson, SD}}
{{509,Campbell, SD},{510,McPherson, SD},{511,Potter, SD},{512,Walworth, SD}}
{{513,Bell, KY},{514,Bland, VA},{515,Cannon, TN},{516,Crockett, TN}}
{{517,Gibson, TN},{518,Madison, TN},{519,Meigs, TN},{520,Moore, TN}}
{{521,Wilson, TN},{522,Anderson, TX},{523,Kenedy, TX},{524,Andrews, TX}}
{{525,Wilson, TX},{526,Crockett, TX},{527,Armstrong, TX},{528,Parmer, TX}}
{{529,Archer, TX},{530,Brooks, TX},{531,Borden, TX},{532,Johnson, TX}}
{{533,Pecos, TX},{534,Willacy, TX},{535,King, TX},{536,Coke, TX}}
{{537,Tarrant, TX},{538,Collin, TX},{539,Bexar, TX},{540,Bastrop, TX}}
{{541,Crosby, TX},{542,Eastland, TX},{543,Hutchinson, TX},{544,Foard, TX}}
{{545,Howard, TX},{546,Guadalupe, TX},{547,Cochran, TX},{548,Hale, TX}}
{{549,San Saba, TX},{550,Hamilton, TX},{551,Jim Hogg, TX},{552,Schleicher, TX}}
{{553,Kent, TX},{554,Lamb, TX},{555,Limestone, TX},{556,Martin, TX}}
{{557,Menard, TX},{558,Motley, TX},{559,Parker, TX},{560,Palo Pinto, TX}}
{{561,San Jacinto, TX},{562,Sterling, TX},{563,Washington, TX},{564,Webb, TX}}
{{565,Zapata, TX},{566,Daggett, UT},{567,Piute, UT},{568,Wayne, UT}}
{{569,Grand Isle, VT},{570,Rappahannock, VA},{571,Appomattox, VA},{572,Campbell, VA}}
{{573,Bedford, VA},{574,Loudoun, VA},{575,Fauquier, VA},{576,Scott, VA}}
{{577,Dickenson, VA},{578,Craig, VA},{579,Hanover, VA},{580,King and Queen, VA}}
{{581,Nelson, VA},{582,Orange, VA},{583,Powhatan, VA},{584,Russell, VA}}
{{585,Surry, VA},{586,Tucker, WV},{587,Wirt, WV},{588,Adams, WI}}
{{589,Buffalo, WI},{590,Crawford, WI},{591,Jefferson, WI},{592,Pierce, WI}}
{{593,Polk, WI},{594,Richland, WI},{595,Sauk, WI},{596,Washburn, WI}}
{{597,Sawyer, WI},{598,Waushara, WI},{599,Teton, ID},{600,Teton, WY}}

**E. Isolated/ungrouped counties having no 1's in either the corresponding row or column**

{{1,St. Clair, AL},{2,Aleutians East, AK},{3,Denali, AK},{4,Haines, AK}}
{{5,Faulkner, AR},{6,San Benito, CA},{7,Yolo, CA},{8,Boulder, CO}}
{{9,Cheyenne, CO},{10,San Juan, CO},{11,Litchfield, CT},{12,St. Johns, FL}}
{{13,Walker, GA},{14,Kalawao, HI},{15,Power, ID},{16,Henry, IL}}
{{17,Kane, IL},{18,Kendall, IL},{19,Mercer, IL},{20,Whiteside, IL}}
{{21,Adams, IN},{22,Dubois, IN},{23,Union, IN},{24,Emmet, IA}}
{{25,Warren, IA},{26,Greeley, KS},{27,Morton, KS},{28,Rice, KS}}
{{29,Stafford, KS},{30,Campbell, KY},{31,Casey, KY},{32,Harrison, KY}}
{{33,Magoffin, KY},{34,Franklin, MA},{35,Monroe, MI},{36,Washtenaw, MI}}
{{37,Holmes, MS},{38,Wilkinson, MS},{39,Daviess, MO},{40,Livingston, MO}}
{{41,Webster, MO},{42,Frontier, NE},{43,Hayes, NE},{44,Nemaha, NE}}
{{45,Sherman, NE},{46,Gloucester, NJ},{47,Mercer, NJ},{48,Hidalgo, NM}}
{{49,Madison, NY},{50,Richmond, NY},{51,Onslow, NC},{52,Divide, ND}}
{{53,Eddy, ND},{54,Emmons, ND},{55,Kidder, ND},{56,Nelson, ND}}
{{57,Ashland, OH},{58,Lawrence, OH},{59,Warren, OH},{60,Beaver, OK}}
{{61,Canadian, OK},{62,Creek, OK},{63,Harper, OK},{64,Lincoln, OK}}
{{65,Rogers, OK},{66,Forest, PA},{67,Sullivan, PA},{68,Washington, PA}}
{{69,Washington, RI},{70,Dorchester, SC},{71,Haakon, SD},{72,Jones, SD}}
{{73,Sully, SD},{74,Chester, TN},{75,Hancock, TN},{76,Humphreys, TN}}
{{77,Tipton, TN},{78,Williamson, TN},{79,Denton, TX},{80,Hansford, TX}}
{{81,Harrison, TX},{82,Loving, TX},{83,McMullen, TX},{84,Montgomery, TX}}
{{85,Starr, TX},{86,Trinity, TX},{87,Beaver, UT},{88,Morgan, UT}}
{{89,Amherst, VA},{90,Buchanan, VA},{91,Buckingham, VA},{92,Floyd, VA}}
{{93,Fluvanna, VA},{94,Highland, VA},{95,Island, WA},{96,Pierce, WA}}
{{97,Barron, WI},{98,Burnett, WI},{99,Calumet, WI},{100,Menominee, WI}}

**F. Largest (three-state) weak component of the 3,007-vertex digraph**

{{1,Butler, KY},{2,Edmonson, KY},{3,Grayson, KY},{4,Simpson, KY}}
{{5,Acadia, LA},{6,St. Landry, LA},{7,Allen, LA},{8,Avoyelles, LA}}
{{9,Pointe Coupee, LA},{10,Beauregard, LA},{11,Calcasieu, LA},{12,Jefferson Davis, LA}}
{{13,Caldwell, LA},{14,La Salle, LA},{15,Cameron, LA},{16,Catahoula, LA}}
{{17,East Feliciana, LA},{18,West Feliciana, LA},{19,Evangeline, LA},{20,Iberia, LA}}
{{21,Vermilion, LA},{22,Iberville, LA},{23,Plaquemines, LA},{24,St. Bernard, LA}}
{{25,West Baton Rouge, LA},{26,Hancock, MS},{27,Vernon, LA},{28,Washington, LA}}
{29,Pearl River, MS}

**G. Second largest (five [intermountain]-state) weak component of the 3,007-vertex digraph**

{{1,Bear Lake, ID},{2,Skamania, WA},{3,Caribou, ID},{4,Clark, ID}}
{{5,Oneida, ID},{6,Churchill, NV},{7,Lyon, NV},{8,Douglas, NV}}
{{9,El Dorado, CA},{10,Lander, NV},{11,Mineral, NV},{12,Washoe, NV}}
{{13,Carson City, NV},{14,Gilliam, OR},{15,Morrow, OR},{16,Grant, OR}}
{{17,Wheeler, OR},{18,Harney, OR},{19,Hood River, OR},{20,Umatilla, OR}}
{{21,Sherman, OR},{22,Walla Walla, WA},{23,Wasco, OR},{24,Columbia, WA}}
{{25,Garfield, WA},{26,Lincoln, WA},{27,Klickitat, WA}}

**H. Third largest (two-state) weak component of the 3,007-vertex digraph**

{{1,Greer, OK},{2,Tillman, OK},{3,Harmon, OK},{4,Jefferson, OK}}
{{5,Clay, TX},{6,Stephens, OK},{7,Bee, TX},{8,Gonzales, TX}}
{{9,Blanco, TX},{10,Scurry, TX},{11,Caldwell, TX},{12,Hays, TX}}
{{13,Castro, TX},{14,Deaf Smith, TX},{15,Chambers, TX},{16,Wichita, TX}}
{{17,Oldham, TX},{18,Liberty, TX},{19,Live Oak, TX},{20,Mason, TX}}
{{21,Matagorda, TX},{22,San Jacinto, TX},{23,Wharton, TX}}

**I. Fourth largest (two-state) weak component of the 3,007-vertex digraph**

{{1,Chicot, AR},{2,Washington, MS},{3,Clark, AR},{4,Grant, AR}}
{{5,Desha, AR},{6,Drew, AR},{7,Jefferson, AR},{8,Lincoln, AR}}
{{9,Pike, AR},{10,Bolivar, MS},{11,Coahoma, MS},{12,Tallahatchie, MS}}
{{13,Humphreys, MS},{14,Yazoo, MS},{15,Issaquena, MS},{16,Panola, MS}}
{{17,Tate, MS},{18,Quitman, MS},{19,Sharkey, MS},{20,Sunflower, MS}}
{{21,Yalobusha, MS},{22,Lafayette, MS}}
